# Supplementary material for: Efficiently Computing Nash Equilibria in Adversarial Team Markov Games
Source: arXiv:2208.02204 source file (2022-08-03)
Supplement: Supplementary file 1 [file convex-nonconvex-set-figure.tex]

%https://tex.stackexchange.com/questions/639115/how-to-draw-convex-strictly-convex-and-nonconvex-sets
\tikzset{
    convexset/.style = {line width = 0.75 pt, fill = orange},
    ext/.style = {circle, inner sep=0pt, minimum size=2pt, fill=black},
    segment/.style = {line width = 0.75 pt}
        }

\begin{tikzpicture}
    \draw[convexset]
            (0,0) .. controls + (0.2,2) and + (-0.2,1) ..
            (3,1) .. controls + (0.2,-0.5) and + (0.5,0) ..
            (1.1,-2) .. controls + (-0.5,0) and + (-0.1,-1) ..
            (0,0) -- cycle;
    \draw[segment] (1,-1) node[ext]{} -- (1.5,1) node[ext]{};
\end{tikzpicture}%
\hspace*{2cm}%  
\begin{tikzpicture}[scale=0.65]
    \draw[convexset]
            (0,0) .. controls + (0.2,0) and +(-1,0) ..
            (1.3,-2) .. controls + (1,0) and + (-0.2,0) ..
            (5,0) .. controls + (0.2,0) and + (1,0) ..
            (2,-7) .. controls + (-1,0) and + (-0.2,0) ..
            (0,0) -- cycle;
    \draw[segment] (0.5,-1.5) node[ext]{} -- (3.5,-1.5) node[ext]{};
\end{tikzpicture}
