# Supplementary material for: Efficiently Computing Nash Equilibria in Adversarial Team Markov Games
Source: arXiv:2208.02204 source file (2022-08-03)
Supplement: Supplementary file 2 [file mpg.tex]

%  \section{Probably-not-useful-for now}
%  \subsection{Independent Learning}
 
%  Agents exist within the framework of a Markov Game and continually execute policies. The goal is for all agents to approach a Nash Equilibrium. Each agent $k$ uses a policy $\pi_k^{(i)} : S \xrightarrow[]{} \Delta(K)$ and observes a different trajectory $(s_1^{(i)},k_1^{(i)},r_1^{(i)}),\dots,(s_T^{(i)},k_T^{(i)},r_T^{(i)})$. Recall, each agent only has knowledge about their own actions.
 
%  \begin{definition}
%     We call a set of algorithms an \textit{independent distributed protocol} if knowledge of the game is obtained through interacting with the environment \textit{(independent oracle)} and all players are only allowed to use private storage, which can only save a finite number of past trajectories \textit{(limited private storage)}.
%  \end{definition}
%  \label{sec:mpg}
 
    A recent strain of research in multi-agent reinforcement learning extends the concept of potential games~\citep{monderer1996potential} to their stochastic variant~\citep{marden2012state,macua2018learning,leonardos2021global}.
